# Supplementary material for: Influence Maximization with Spontaneous User Adoption
Source: arXiv:1906.02296 source file (2020-03-11)
Supplement: Supplementary file 1 [file appendix_old.tex]

\appendix

\section*{Appendix}
The appendix is organized as follows.
In Section~\ref{app:proofs}, we give all proofs of lemmas and theorems , i.e.,
Section~\ref{app:namrim} for the non-adaptive MRIM, 
Section~\ref{app:amrim} for the adaptive MRIM,
Section~\ref{app:crimm} for the \BIM,
and Section~\ref{app:wrimm} for the \BIM,
%and Section~\ref{app:imm} for scalable implementations.
In Section~\ref{app:pseudocode}, we give our complete IMM algorithms and compare them with the original IMM.


\section{Preliminaries} 


\begin{algorithm}[t] 
	\caption{{SABNS}: Unique Activation with Activation Boost Node Selection} \label{alg:crnr}
	\KwIn{RR sets $\cR$, $k$, $p$, $r$}
	%	\KwIn{\newalg{[from round $i-1$] all active nodes by round $i-1$
	%			$A_{i-1}$, newly activated nodes $A^{\new}_{i-1}$, adaptive RR-sets
	%			$\cR_{i-1}$ , optimal value lower bound threshold $x_{i-1}$}}
	\KwOut{seed sets $S^o$}
	
	
	$S^o \leftarrow \emptyset$; 
	$\theta \leftarrow |\cR|$\;
	$\cR'[1...\theta] \leftarrow \emptyset$;
	$numerator[1...\theta] \leftarrow 0$;$denominator[1...\theta] \leftarrow 0$\; 
	\For{$i = 1 \; to \; \theta$}{
		%$R' \leftarrow \{u \in R \mid random(0,1) < p[u]\}$\;
		\For{$u \in \cR[i]$}
		{	
			% $\cR'[i] \leftarrow \emptyset$\;
			\If{$random(0,1) < p[u]$}
			{	$\cR'[i] \leftarrow \cR'[i] \cup \{u\}$\;
				$denominator[i] += r[u]$\;}
		}
		%$\cR' \leftarrow \cR' \cup R'$
	}
	$Indice[V]$ stores index of RR set for each node\;
	\For{$i = 1 \; to \; k$ \label{line:crfor1}}{
		$score[1...\theta] \leftarrow 0$\;
		\For{$u \in V \setminus S^o$}{
			$tmp\_num, tmp\_denom \leftarrow 0$\;
			\For{$j \in Indice[u]$ }{
				$tmp\_num = numerator[j] + r[u]$\;
				\If{$u \in \cR[j]$ and $u \notin \cR'[j]$}
				{$tmp\_denom =denominator[j] + r[u]$}
				$score[u] += tmp\_num/tmp\_denom$\;
			}
		}
		
		%\For{$i = 1 \; to \; k$ \label{line:crfor1}}{
		$u \leftarrow \argmax_{u'\in V \setminus S^o} score[u']$\;
		$S^o \leftarrow S^o \cup \{u\}$\;
		%}
		\For{$j \in Indice[u]$ }{
			$numerator[j] += r[u]$\;
			\If{$u \in \cR[j]$ and $u \notin \cR'[j]$}
			{$denominator[j] += r[u]$\;
				$\cR'[j] \leftarrow \cR'[j] \cup \{u\}$\;
			}
		}
	}
	\bf{return} $S^o $.
\end{algorithm}

\subsection{Algorithm for Boost Centrality}
\begin{algorithm}[t] 
	%\SetKwComment{tcp}{\tiny // }{}%
	\caption{{BC}: Node Marginal Influence} \label{alg:sasni}
	\KwIn{Graph $G=(V,E, p)$, Parameters: random triggering set distribution $\{T(v)\}_{v\in V} , \epsilon > 0, l > 0, k \in [n]$}
	\KwOut{$\hat{\psi}_v$, $\forall v \in V$: estimated centrality measure.}
	
	\tcp{Phase 1: Estimating the number of RR sets needed, $\theta$}
	$LB \leftarrow 1$; $\varepsilon' = \sqrt{2}$; $\theta_0 = 0$\;
	$est_v = 0$ for every $v \in V$\;
	\For{$i = 1$ to $\lfloor\log_2{n}\rfloor - 1$}{
		$x \leftarrow \newalg{n}/2^i$\; \label{line:assignx}
		$\theta_i = \frac{n\cdot((l+1)\ln\log_2{n}+\ln{2})\cdot(2+\frac{2}{3}\epsilon')}{{\epsilon'}^2\cdot x}$\;
		\For{$j = 1$  to  $\theta_i - \theta_{i-1}$ \label{line:for1}}{
			generate a random RR set $R$\; \label{line:genRRset1a}
			\For{$v \in R$ \label{line:for2}}{
				for every $u \in R$, remove $u$ in $R \setminus \{v\}$, while random simulate number $\mu> p_u$, $\mu \in [0,1]$\;
				if $|R| == 1$, $est_v = est_v + 1$
			}
		}
		$est^{(k)}$ = the k-th largest value in $\{est_v\}_{v \in V}$\;
		\If{$n \cdot est^{(k)} \geq (1 + \epsilon') \cdot x$}{
			\label{line:estimate1}
			$LB \leftarrow \newalg{ n \cdot est^{(k)}/(\theta_i \cdot (1 + \epsilon'))}$\; 
			\label{line:estimate2}
			break\;
		} 
	}
	\tcp{Phase 2: Estimate NMI}
	$est_v = 0$ for every $v \in V$\;
	\For{$j = 1$ to $\theta$}{
		generate a random RR set $R$\; \label{line:genRRset1a}
		\For{$v \in R$ \label{line:for2}}{
			for every $u \in R$, remove $u$ in $R \setminus \{v\}$, while random simulate number $\mu> p_u$, $\mu \in [0,1]$\;
			if $|R| == 1$, $est_v = est_v + 1$
		}
	}
	for every $v \in V$ , $\hat{\psi}^v = n \cdot est_v / \theta$\;
	\bf{return} $\hat{\psi}^v$, $v \in V$.
\end{algorithm}

\subsection{Social Influence Models}
A network-influence instance is usually specified by a triple $\cI = (V, E, P_{\cI})$, 
where a directed graph $G = (V, E)$ represents the structure of a social network,
$V$ is a finite set of vertices or nodes, 
$E \subseteq V \times V$ is the set of directed edges connecting pairs of nodes, 
and $P_{\cI}$ defines the influence model.

In this paper, we focus on the well-studied {\em triggering model} \cite{kempe03} as the basic diffusion model.
The diffusion of information or influence proceeds in discrete time steps $\tau = 0, 1, 2, \dots$. 
At time $\tau=0$, the {\em seed set} $S_0$ is selected to be active, and also 
each node $v$ independently chooses a random {\em triggering set} $T(v)$ 
according to some distribution over subsets of its in-neighbors. 
At each time $\tau \ge 1$, an inactive node $v$ becomes active if at least 
one node in $T(v)$  is active by time $\tau-1$. %($u\in S^{(\tau-1)}$).
The diffusion process ends when there is no more nodes activated in a time step.
We remark that the classical Independent Cascade (IC) model is a special case of the triggering model.
In the IC model, 
every edge $(u,v) \in E$ is associated with a probability $q_{uv} \in [0, 1]$, 
and $q_{uv}$ is set to zero if $(u,v) \notin E$.
Each triggering set $T(v)$ is generated by independently sampling $(u,v)$ with probability $q_{uv}$
and including $u$ in $T(v)$ if the sampling of $(u,v)$ is successful.

The triggering model can be equivalently described as propagations in {\em live-edge graphs}.
Given a class of triggering sets $\{T(v)\}_{v\in V}$, we can construct the live-edge graph
$L = (V, E(L))$, where $E(L) = \{(u,v) \mid v\in V, u\in T(v)\}$, and
each edge $(u,v)\in L$ is called a {\em live edge}.
It is easy to see that the propagation in the triggering model is the same as the deterministic
propagation in the corresponding live-edge graph $L$: if $A$ is the set of active nodes
at time $\tau-1$, then all directed out-neighbors of nodes in $A$ will be active
by time $\tau$.
An important metric in any diffusion model is the {\em influence spread},
the expected number of active nodes when the propagation from the given  
seed set $S_0$ ends, denoted as $\sigma(S_0)$.
Let $\Gamma(G,S)$ denote the set of nodes in graph $G$ that can be reached from the node set $S$.
Then, by the above equivalent live-edge graph model, we have
$\sigma(S_0) = \E[|\Gamma(L,S_0)|]$, 
where the expectation is taken over the distribution of live-edge graphs. 

A set function $f:V\rightarrow \R$ is called {\em submodular} if
for all $S  \subseteq O  \subseteq V$ and $u \in V\setminus T$, 
$f(S \cup \{u\}) - f(S) \ge f(O \cup \{u\}) - f(O)$.
Intuitively, submodularity characterizes the diminishing return property often occurring
in economics and operation research.
Moreover, a set function $f$ is called {\em monotone} if for all $S \subseteq O \subseteq V$, $f(S) \le f(O)$.
It is shown in~\cite{kempe03} that influence spread $\sigma$ for the triggering model
is a monotone submodular function .
A non-negative monotone submodular function allows a greedy solution to
its maximization problem subject to a cardinality constraint, with an
approximation ratio $1-1/e$, where $e$ is the base of the natural logarithm~\cite{NWF78}.
This is the technical foundation for most influence maximization tasks.

More generally, we define an influence instance as a triple $\cI = (V, E, P_{\cI})$, 
where $G = (V, E)$ represents the underlying network, 
and $P_{\cI}: 2^V \times 2^V \rightarrow \R$ defines the probability that in the influence process, 
any seed set $S \subseteq V$ activates exactly nodes in any target set $T \subseteq V$ and no other nodes:
If $I_{\cI}(S)$ denotes the random set activated by seed set $S$,
then $Pr(I_{\cI}(S) = T) = P_{\cI}(S, T)$. 
This probability profile is commonly defined by a succinct influence model, 
such as the triggering model, which interacts with network G. 
We also require that: (a) $P_{\cI}(\emptyset, \emptyset) = 1$, 
$P_{\cI}(\emptyset, T) = 0$, $\forall T \neq \emptyset$,
and (b) if $S \nsubseteq T$ then $P_{\cI}(S, T) = 0$, 
i.e., $S$ always activates itself ($S \subseteq I_{\cI}(S)$). 
Such model is also referred to as the progressive influence model. 
The influence spread of $S$ is:
\begin{equation*}
\sigma_{\cI}(S) = \E [|I_{\cI}(S)|] = \sum_{T \subseteq V, S \subseteq T} P_{\cI}(S, T) \cdot |T|. 
\end{equation*}

\subsection{Coalitional Games and Shapley Values}
An $n$-person coalitional game over V = [n] is specified by a characteristic function $\gamma$: 
$2^{|V|} \leftarrow \R$,
where for any coalition $S \subseteq V$,
$\gamma(S)$ denotes the cooperative utility of $S$.
In cooperative game theory,
a ranking function $\theta$ is a mapping from a characteristic function $\gamma$ to a vector in $\R^n$.
A fundamental solution concept of cooperative game theory is the ranking
function given by the Shapley value [31]:
Let $\Pi$ be the set of all permutations of $V$.
For any $v \in V$ and $\pi \in \Pi$,
let $S_{\pi, v}$ denote the set of nodes in $V$ preceding $v$ in permutation $\pi$.
Then, $\forall v \in V$:
\begin{align*}
\phi_{v}^{Shapley}(\gamma) 
&= \frac{1}{n!} \sum_{\pi \in \Pi} (\gamma(S_{\pi, v} \cup \{v\}) - \gamma(S_{\pi, v})) \\
&= \sum_{S \subseteq V \setminus \{v\}} \frac{|S|!(n-|S|-1)!}{n!} (\gamma(S \cup \{v\}) - \gamma(S)).
\end{align*}
We use $\pi \sim \Pi$ to denote that $\pi$ is a random permutation uniformly drawn from $\Pi$.
Then:
\begin{equation*}
\phi_{v}^{Shapley}(\gamma)  = \E_{\pi \sim \Pi} [\gamma(S_{\pi, v} \cup \{v\}) - \gamma(S_{\pi, v})].
\end{equation*}
The Shapley value of $v$ measures $v$'s marginal contribution over the set preceding $v$ in a random permutation.


\section{Algorithms} \label{app:pseudocode}

\subsection{Non-Boost Influence Maximization Algorithm}
%\alg{\WRIMM} (Algorithm \ref{alg:wrimm})  contains two main phases like standard \alg{IMM}.
In Phase 1, the algorithm estimates the number of RR sets $\theta$  needed by estimating
the lower bound $LB$ of the optimal influence spread.
It is done by iteratively halving a threshold value $x_t$, and for each
$x_t$ value, generating $\theta_j$ RR sets (lines~\ref{line:wgenRRset1b}--\ref{line:wgenRRset1e}),
and finding the seed set $\cS_j$ from the current RR sets (line~\ref{line:wnodeselect1}), 
and checking if the current $x_t$ is good enough for the lower bound estimate
(line~\ref{line:wcheckLB}), where $F_{M}(\cS_j)$ is the fraction of RR sets
in $\cM$ that are covered by $\cS_j$.
Procedure $\alg{NodeSelection}(\cM,k)$ is to greedily select $k$ nodes that covers
the most number of RR sets in $\cM$, and it is the same as in~\cite{tang15}, so it
is omitted.
In Phase 2, based on the $\theta$ RR sets generated, $\cS_t$ can be selected
by procedure $\alg{NodeSelection}(\cM,k)$.
Finally, propagation from $\cS_t$ are observed and the active nodes are used as the
feedback for the next round.


Therefore, with Eq.~\eqref{eq:AdaRRset}, the same RR-set based algorithm can be used,
and we only need to properly change the RR-set generation process and the
estimation process.
Algorithm~\ref{alg:aimm} provides the pseudocode for the \alg{AdaIMM} algorithm, which
is based on the \alg{IMM} algorithm in~\cite{tang15}.
For convenience, we mark the part different from \alg{IMM} in blue.
Phase 1 of the algorithm estimate the number $\theta$ of RR sets needed by estimating
the lower bound $LB$ of the optimal spread value.
This estimation is by iteratively halving a threshold value $x_t$, and for each
$x_t$ value, generate $\theta_j$ RR sets (lines~\ref{line:genRRset1b}--\ref{line:genRRset1e}),
and find the seed set $S_j$ from the current RR sets (line~\ref{line:nodeselect1}), 
and check
if the current $x_t$ is good enough for the lower bound estimate
(line~\ref{line:checkLB}), where $F_{M}(S_j)$ is the fraction of RR sets
in $M$ that are covered by $S_j$.
Procedure $\alg{NodeSelection}(M,k)$ is to greedily select $k$ nodes that covers
the most number of RR sets in $M$, and it is the same as in~\cite{tang15}, so it
is omitted.
In Phase 2, $\theta$ RR sets are generated and node $S_t$ is selected greedily
by procedure $\alg{NodeSelection}(M,k)$.
Finally, propagation from $S_t$ are observed and the activated nodes are used as the
feedback for the next round.

The main differences from the standard \alg{IMM} include several points.
First, whenever we generate new RR sets in round $t$, we only start from roots in
$V \setminus A_{t-1}$ (lines~\ref{line:sample1} and~\ref{line:sample2}), as explained by Lemma~\ref{lem:ARRset}.
Second, when we estimate the influence spread, we need to adjust it using
$n_a = n - |A_{t-1}|$ (lines~\ref{line:for1}, \ref{line:assignx}, \ref{line:estimate1}, \ref{line:estimate2}),
again by Lemma~\ref{lem:ARRset}.
Third, we need to adjust $\ell$ to be $\ell + \log(2T)/\log n$,
and $\varepsilon$ to $\varepsilon_0 = e^{(1-1/e)} \varepsilon/2$.
This is to guarantee that in each round we have probability at least $1 - 1/(n^\ell T)$ to
have $S_t$ as a $(1-1/e - \varepsilon_0)$ approximation, so that the result for the
total $T$ rounds would come out correctly as stated in the following theorem.

\begin{algorithm}[t] 
	\caption{{SAO}:Overall Marginal Influence with Activation Boost IMM algorithm
	} \label{alg:saonw}
	\KwIn{Graph $G=(V,E)$, budget $k$, self-activation probability $p$, accuracy parameters $(\varepsilon, \ell)$, triggering set distributions}
	\KwOut{seed set $S$}
	
	\tcp{Phase 1: Estimating the number of RR sets needed, $\theta$}
	$\newalg{\ell \leftarrow \ell + \ln 2 / \ln{n}} $;
	$\newalg{\cR \leftarrow \emptyset}$;  $LB \leftarrow 1$; $\varepsilon' \leftarrow \sqrt{2}\varepsilon$\;
	$\alpha \leftarrow \sqrt{\ell \ln{n} + \ln{2}}$;
	$\beta \leftarrow \sqrt{(1-1/e)\cdot (\ln{\binom{n}{k}}+\alpha^2)}$\;
	$\lambda' \leftarrow [(2+\frac{2}{3}\varepsilon') \cdot (\ln{{\binom{n}{k}}}+\ell \cdot \ln{n}+\ln{\log_2{n}})\cdot n]/\varepsilon'^2$\;
	$\lambda^* \leftarrow 2 n \cdot ((1-1/e) \cdot \alpha + \beta)^2 \cdot \varepsilon^{-2}$\;
	
	\For{$i = 1 \; to \; \log_2{(\newalg{n} - 1)}$ \label{line:cfor1}}{
		$x \leftarrow \newalg{n}/2^i$\; \label{line:cassignx}
		$\theta_i \leftarrow \lambda'/x_i$\; \label{line:cgenRRset1b} 
		\While{$\newalg{|\cR|}< \theta_i$}{
			Select a node $u$ from $V$ uniformly at random\; \label{line:csample1}
			Generate RR-vector $\newalg{R}$ from $u$, and insert it into $\newalg{\cR}$ only if any $v \in R$ is not activated by its self-activation probability $p$\;  \label{line:cgsample1}
		}\label{line:cgenRRset1e} 
		\newalg{$S_i \leftarrow \NS(\cR, k)$}\; \label{line:cnodeselect1}
		\If{$\newalg{n} \cdot \newalg{F_{\cR}(S_i)} \geq (1 + \varepsilon') \cdot x$}{
			\label{line:cestimate1}
			$LB \leftarrow \newalg{n} \cdot \newalg{F_{\cR}(S_i)}/(1 + \varepsilon')$\; 
			\label{line:cestimate2}
			break\;
		} 
	}
	$\theta \leftarrow \lambda^* / LB$\;
	\While{$\newalg{|\cR|} \leq \theta$}{ \label{line:ccheckLB}
		Select a node $u$ from $V$  uniformly at random\;\label{line:csample2}
		Generate \newalg{$R$} for $u$,
		and insert it into \newalg{$\cR$} only if any $v \in R$ is not activated by its self-activation probability $p$\; \label{line:cgsample2}		
	}
	\tcp{Phase 2: Generate $\theta$ RR-vector sets and select seed nodes}
	%\{Phase 2: Generate $\theta$ RR-vector sets and select seed nodes\}\;
	\newalg{$S \leftarrow \NS(\cR, k)$}\;
	
	\bf{return} $S$.
\end{algorithm}

\subsection{Boost Influence Maximization Algorithm}
%\alg{\WRIMM} (Algorithm \ref{alg:wrimm})  contains two main phases like standard \alg{IMM}.
In Phase 1, the algorithm estimates the number of RR sets $\theta$  needed by estimating
the lower bound $LB$ of the optimal influence spread.
It is done by iteratively halving a threshold value $x_t$, and for each
$x_t$ value, generating $\theta_j$ RR sets (lines~\ref{line:wgenRRset1b}--\ref{line:wgenRRset1e}),
and finding the seed set $\cS_j$ from the current RR sets (line~\ref{line:wnodeselect1}), 
and checking if the current $x_t$ is good enough for the lower bound estimate
(line~\ref{line:wcheckLB}), where $F_{M}(\cS_j)$ is the fraction of RR sets
in $\cM$ that are covered by $\cS_j$.
Procedure $\alg{NodeSelection}(\cM,k)$ is to greedily select $k$ nodes that covers
the most number of RR sets in $\cM$, and it is the same as in~\cite{tang15}, so it
is omitted.
In Phase 2, based on the $\theta$ RR sets generated, $\cS_t$ can be selected
by procedure $\alg{NodeSelection}(\cM,k)$.
Finally, propagation from $\cS_t$ are observed and the active nodes are used as the
feedback for the next round.


Therefore, with Eq.~\eqref{eq:AdaRRset}, the same RR-set based algorithm can be used,
and we only need to properly change the RR-set generation process and the
estimation process.
Algorithm~\ref{alg:aimm} provides the pseudocode for the \alg{AdaIMM} algorithm, which
is based on the \alg{IMM} algorithm in~\cite{tang15}.
For convenience, we mark the part different from \alg{IMM} in blue.
Phase 1 of the algorithm estimate the number $\theta$ of RR sets needed by estimating
the lower bound $LB$ of the optimal spread value.
This estimation is by iteratively halving a threshold value $x_t$, and for each
$x_t$ value, generate $\theta_j$ RR sets (lines~\ref{line:genRRset1b}--\ref{line:genRRset1e}),
and find the seed set $S_j$ from the current RR sets (line~\ref{line:nodeselect1}), 
and check
if the current $x_t$ is good enough for the lower bound estimate
(line~\ref{line:checkLB}), where $F_{M}(S_j)$ is the fraction of RR sets
in $M$ that are covered by $S_j$.
Procedure $\alg{NodeSelection}(M,k)$ is to greedily select $k$ nodes that covers
the most number of RR sets in $M$, and it is the same as in~\cite{tang15}, so it
is omitted.
In Phase 2, $\theta$ RR sets are generated and node $S_t$ is selected greedily
by procedure $\alg{NodeSelection}(M,k)$.
Finally, propagation from $S_t$ are observed and the activated nodes are used as the
feedback for the next round.

The main differences from the standard \alg{IMM} include several points.
First, whenever we generate new RR sets in round $t$, we only start from roots in
$V \setminus A_{t-1}$ (lines~\ref{line:sample1} and~\ref{line:sample2}), as explained by Lemma~\ref{lem:ARRset}.
Second, when we estimate the influence spread, we need to adjust it using
$n_a = n - |A_{t-1}|$ (lines~\ref{line:for1}, \ref{line:assignx}, \ref{line:estimate1}, \ref{line:estimate2}),
again by Lemma~\ref{lem:ARRset}.
Third, we need to adjust $\ell$ to be $\ell + \log(2T)/\log n$,
and $\varepsilon$ to $\varepsilon_0 = e^{(1-1/e)} \varepsilon/2$.
This is to guarantee that in each round we have probability at least $1 - 1/(n^\ell T)$ to
have $S_t$ as a $(1-1/e - \varepsilon_0)$ approximation, so that the result for the
total $T$ rounds would come out correctly as stated in the following theorem.

\section{Proofs for Lemmas and Theorems}\label{app:proofs}

\subsection{Proofs for Section \ref{sec:nonadaptive} [Boosted Influence Maximization]}\label{app:bim}

%\bmonotone*
%\begin{proof}
%	Equivalently, the monotonicity of influence spread function $\rho_s(\cdot)$ can be transferred as:
%	For any $S \subseteq V$ and $v \in V \setminus S$, we have $\rho_s(S) \leq \rho_s(S \cup \{v\}) \Leftrightarrow  \rho_s(S \cup \{v\})-\rho_s(S) \geq 0$.
%	
%	According to the definition of the influence spread, we have two situations by arriving time:
%	\begin{itemize}
%		\item Additional node $v$'s arrival time is later than all $S$. By Eq.~\ref{eq:spreadfunction5}, the influence of $S$ would not change and $v$ can produce non-negative marginal contribution. Then, we can easily have $\rho_s(S) \leq \rho_s(S \cup \{v\})$.
%		\item Additional node $v$'s arrival time is earlier than at least a node $u \in S$. Let use $S_{\pi(p), u}$ indicates the set of nodes in $V$ preceding $u$ in permutation $\pi(p)$. Due to we have the additional seed $v \in S_{\pi(p), u}$, indicating less number of activated nodes by $S_{\pi(p), u} \cup \{u\} \setminus S$, we have $\rho_s(S) \leq \rho_s(S \cup \{v\})$. 
%	\end{itemize}	
%	
%	Thus the monotonicity holds.
%\end{proof}


%\bsubmodular*
%\begin{proof}
%	According to the definition of the influence spread, we have
%	\begin{align*}
%	&\rho_s(S^A \cup \{u\}) - \rho_s(S^A) \geq \rho_s(S^B \cup \{u\})-\rho_s(S^B) \\
%	\Leftrightarrow & \E_{\pi \in \Pi(r)}\left[ E_L[|\bigcup_{u \in S^A \cup \{u\}} \Gamma(L, S_{\pi(p), u} \cup \{u\}) \setminus \Gamma(L, S_{\pi(p), u})|] \right] \\
%	& - \E_{\pi \in \Pi(r)}\left[ E_L[|\bigcup_{u \in S^A} \Gamma(L, S_{\pi(p), u} \cup \{u\}) \setminus \Gamma(L, S_{\pi(p), u})|] \right] \\
%	\geq & \E_{\pi \in \Pi(r)}\left[ E_L[|\bigcup_{u \in S^B \cup \{u\}} \Gamma(L, S_{\pi(p), u} \cup \{u\}) \setminus \Gamma(L, S_{\pi(p), u})|] \right] \\
%	& - \E_{\pi \in \Pi(r)}\left[ E_L[|\bigcup_{u \in S^B} \Gamma(L, S_{\pi(p), u} \cup \{u\}) \setminus \Gamma(L, S_{\pi(p), u})|] \right] \\
%	\end{align*}
%	Then it is sufficient to show that
%	\begin{align*}
%	& \bigcup_{u \in S^A \cup \{u\}} \Gamma(L, S_{\pi(p), u} \cup \{u\}) 
%	\setminus \bigcup_{u \in S^A} \Gamma(L, S_{\pi(p), u} \cup \{u\}) \setminus \Gamma(L, S_{\pi(p), u}) \\ 
%	\supseteq & \bigcup_{u \in S^B \cup \{u\}} \Gamma(L, S_{\pi(p), u} \cup \{u\})
%	\setminus \bigcup_{u \in S^B} \Gamma(L, S_{\pi(p), u} \cup \{u\}) \setminus \Gamma(L, S_{\pi(p), u}) \\
%	\end{align*}
%	
%	For a node $v \in \bigcup_{u \in S^B \cup \{u\}} \Gamma(L, S_{\pi(p), u} \cup \{u\}) \setminus \bigcup_{u \in S^B} \Gamma(L, S_{\pi(p), u} \cup \{u\}) \setminus \Gamma(L, S_{\pi(p), u}) $, 
%	$v$ is reachable from $\bigcup_{u \in S^B \cup \{u\}} \Gamma(L, S_{\pi(p), u} \cup \{u\})$ in $L$, 
%	but not reachable from $\bigcup_{u \in S^B} \Gamma(L, S_{\pi(p), u} \cup \{u\}) $ in $L$.
%	Thus $v$ is also not reachable from $\bigcup_{u \in S^A} \Gamma(L, S_{\pi(p), u} \cup \{u\}) $ in $L$.
%	Therefore, we conclude that $u \in \bigcup_{u \in S^A \cup \{u\}} \Gamma(L, S_{\pi(p), u} \cup \{u\}) \setminus \bigcup_{u \in S^A} \Gamma(L, S_{\pi(p), u} \cup \{u\}) \setminus \Gamma(L, S_{\pi(p), u})$.
%	Thus the submodularity holds.
%\end{proof}


\subsection{Proofs for Section \ref{sec:nonadaptive} [Preemptive Influence Maximization]}\label{app:pim}

%\padd*
\begin{proof}
	\begin{align*}\label{eq:sumequal}
	\rho(S, p, r) 
	&= \E_{\pi \in \Pi(r)}\left[ E_L[|\bigcup_{u \in S} \Gamma(L, S_{\pi(p), u} \cup \{u\}) \setminus \Gamma(L, S_{\pi(p), u})|] \right] \\
	&= \E_{\pi \in \Pi(r)}\left[ \sum_{u \in S} E_L[ |\Gamma(L, S_{\pi(p), u} \cup \{u\}) \setminus \Gamma(L, S_{\pi(p), u})|] \right] \\
	&= \sum_{u \in S} \E_{\pi \in \Pi(r)}\left[ E_L[ |\Gamma(L, S_{\pi(p), u} \cup \{u\}) \setminus \Gamma(L, S_{\pi(p), u})|] \right] \\	
	&= \sum_{u \in S} \rho(u, p, r)
	\end{align*}
	Thus, the normalization holds.
\end{proof}

\subsection{Proofs for Section \ref{sec:nonadaptive} [Boosted Preemptive Influence Maximization]}\label{app:bpim}

%\alg{\NBIM} is very similar to standard \alg{IMM} and only has a few differences include several points.
We have talked about them in the formal paper already. 


%\bpmonotone*
\begin{proof}
	Equivalently, the monotonicity of influence spread function $\rho_s(\cdot)$ can be transferred as:
	For any $S \subseteq V$ and $v \in V \setminus S$, we have $\rho_s(S) \leq \rho_s(S \cup \{v\}) \Leftrightarrow  \rho_s(S \cup \{v\})-\rho_s(S) \geq 0$.
	
	According to the definition of the influence spread, we have two situations by arriving time:
	\begin{itemize}
		\item Additional node $v$'s arrival time is later than all $S$. By Eq.~\ref{eq:spreadfunction5}, the influence of $S$ would not change and $v$ can produce non-negative marginal contribution. Then, we can easily have $\rho_s(S) \leq \rho_s(S \cup \{v\})$.
		\item Additional node $v$'s arrival time is earlier than at least a node $u \in S$. Let use $S_{\pi(p), u}$ indicates the set of nodes in $V$ preceding $u$ in permutation $\pi(p)$. Due to we have the additional seed $v \in S_{\pi(p), u}$, indicating less number of activated nodes by $S_{\pi(p), u} \cup \{u\} \setminus S$, we have $\rho_s(S) \leq \rho_s(S \cup \{v\})$. 
	\end{itemize}	
	
	Thus the monotonicity holds.
\end{proof}


%\bpsubmodular*
\begin{proof}
	According to the definition of the influence spread, we have
	\begin{align*}
	&\rho_s(S^A \cup \{u\}) - \rho_s(S^A) \geq \rho_s(S^B \cup \{u\})-\rho_s(S^B) \\
	\Leftrightarrow & \E_{\pi \in \Pi(r)}\left[ E_L[|\bigcup_{u \in S^A \cup \{u\}} \Gamma(L, S_{\pi(p), u} \cup \{u\}) \setminus \Gamma(L, S_{\pi(p), u})|] \right] \\
	& - \E_{\pi \in \Pi(r)}\left[ E_L[|\bigcup_{u \in S^A} \Gamma(L, S_{\pi(p), u} \cup \{u\}) \setminus \Gamma(L, S_{\pi(p), u})|] \right] \\
	\geq & \E_{\pi \in \Pi(r)}\left[ E_L[|\bigcup_{u \in S^B \cup \{u\}} \Gamma(L, S_{\pi(p), u} \cup \{u\}) \setminus \Gamma(L, S_{\pi(p), u})|] \right] \\
	& - \E_{\pi \in \Pi(r)}\left[ E_L[|\bigcup_{u \in S^B} \Gamma(L, S_{\pi(p), u} \cup \{u\}) \setminus \Gamma(L, S_{\pi(p), u})|] \right] \\
	\end{align*}
	Then it is sufficient to show that
	\begin{align*}
	& \bigcup_{u \in S^A \cup \{u\}} \Gamma(L, S_{\pi(p), u} \cup \{u\}) 
	\setminus \bigcup_{u \in S^A} \Gamma(L, S_{\pi(p), u} \cup \{u\}) \setminus \Gamma(L, S_{\pi(p), u}) \\ 
	\supseteq & \bigcup_{u \in S^B \cup \{u\}} \Gamma(L, S_{\pi(p), u} \cup \{u\})
	\setminus \bigcup_{u \in S^B} \Gamma(L, S_{\pi(p), u} \cup \{u\}) \setminus \Gamma(L, S_{\pi(p), u}) \\
	\end{align*}
	
	For a node $v \in \bigcup_{u \in S^B \cup \{u\}} \Gamma(L, S_{\pi(p), u} \cup \{u\}) \setminus \bigcup_{u \in S^B} \Gamma(L, S_{\pi(p), u} \cup \{u\}) \setminus \Gamma(L, S_{\pi(p), u}) $, 
	$v$ is reachable from $\bigcup_{u \in S^B \cup \{u\}} \Gamma(L, S_{\pi(p), u} \cup \{u\})$ in $L$, 
	but not reachable from $\bigcup_{u \in S^B} \Gamma(L, S_{\pi(p), u} \cup \{u\}) $ in $L$.
	Thus $v$ is also not reachable from $\bigcup_{u \in S^A} \Gamma(L, S_{\pi(p), u} \cup \{u\}) $ in $L$.
	Therefore, we conclude that $u \in \bigcup_{u \in S^A \cup \{u\}} \Gamma(L, S_{\pi(p), u} \cup \{u\}) \setminus \bigcup_{u \in S^A} \Gamma(L, S_{\pi(p), u} \cup \{u\}) \setminus \Gamma(L, S_{\pi(p), u})$.
	Thus the submodularity holds.
\end{proof}
